# Supplementary material for: Entanglement and Quantum Error Correction with Superconducting Qubits
Source: arXiv:1311.6759 source file (2013-11-26)
Supplement: Supplementary file 1 [file MathematicaCodeAppendix_LR.pdf]

# Definitons

We begin by defining our language, including raising and lowering operators, dagger, tensor product, and Pauli operators. We then make functions to create and manipulate single-qubit states, which generalize to two qubits. We also define a function to produce a Pauli tomogram from a density matrix and $\beta$ and $\kappa$ matrices for converting state tomograms into $\chi$ process matrices.

In[1]:=

```
Needs["BarCharts`"]

ident[dim_] :=
  SparseArray[{{Poutine$_, Poutine$_} -> 1}, {dim, dim}];

destroy[dim_] := SparseArray[{Poutine$_, Maudite$_} /;
   Poutine$ + 1 == Maudite$ -> Sqrt[Poutine$], {dim, dim}];

dagger[a_] := ConjugateTranspose[a];
(*Transpose[Conjugate[a]]; *)

TensProd[a_, b_] := SparseArray[KroneckerProduct[a, b]];
```

General::obspkg :
BarCharts` is now obsolete. The legacy version being loaded may conflict with current Mathematica functionality. See the Compatibility Guide for updating information.

```
In[6]:= σp = destroy[2];
σm = dagger[σp];
σx = σp + σm;
σy = -1 * (-ⅈ σp + ⅈ σm); (* -ⅈ* *)
σz = - σm.σp + σp.σm;
σi = ident[2];

σii = TensProd[σi, σi];
σxi = TensProd[σx, σi];
σyi = TensProd[σy, σi];
σzi = TensProd[σz, σi];

σix = TensProd[σi, σx];
σxx = TensProd[σx, σx];
σyx = TensProd[σy, σx];
σzx = TensProd[σz, σx];

σiy = TensProd[σi, σy];
σxy = TensProd[σx, σy];
σyy = TensProd[σy, σy];
σzy = TensProd[σz, σy];

σiz = TensProd[σi, σz];
σxz = TensProd[σx, σz];
σyz = TensProd[σy, σz];
σzz = TensProd[σz, σz];

DistributeDefinitions[σx, σy, σz, σi, σii, σxi, σyi, σzi,
  σix, σxx, σyx, σzx, σiy, σxy, σyy, σzy, σiz, σxz, σyz, σzz];
U[θ_, σ_] := MatrixExp[-ⅈ θ/2 Normal[σ]];

In[30]:= (* Make a one qubit density matrix with QId,
X90p, Y90p, or Xp rotations on the qubits *)
makeρ1[state_] := Module[{o1},
   ρ = (σi + σz) / 2; (* start from the ground state *)

   o1 = Switch[Characters[state][[1]],
     "I", U[0, σi],
     "X", U[π / 2, σx],
     "Y", U[π / 2, σy],
     "Z", U[π, σx],
     _, U[0, σi]];

   Return[dagger[o1].ρ.o1];
  ];

(* Get Pauli correlations from density matrix *)
paulitomo1[ρ_] := {Tr[ρ.σi], Tr[ρ.σx], Tr[ρ.σy], Tr[ρ.σz]} / 2;
```

```
In[32]:= (* Programmatically create some order of states and operators *)
getorder1[] := Module[{basis},
   basis = {"I", "X", "Y", "Z"};
   basis
  ];

(* Give the density matrix of the kth state in our basis *)
states1 = getorder1[];
state1[k_] := Module[{},
   makeρ1[states1[[k]]]
  ];

(* Give the jth operator in our basis *)
operator1[j_] := Module[{op},
   op = ToExpression["σ" <> ToLowerCase[states1[[j]]]];
   Return[op];
  ];

(* Calculate the β matrix as a 2nd rank tensor for 1 qubit*)
Calcβ1d[] :=
  Module[{j, k, m, n, ii, β, opk, statej, opmstatej, norm, nops},
   β = ConstantArray[0, {2^4, 2^4}];

   nops = Table[0, {ii, 1, 4}];
   For[ii = 1, ii ≤ 4, ii++,
    nops[[ii]] = operator1[ii];
   ];

   For[j = 1, j ≤ 4, j++,
    statej = state1[j];
    For[m = 1, m ≤ 4, m++,
     opmstatej = operator1[m].statej;

     For[k = 1, k ≤ 4, k++,
      opk = Flatten[operator1[k]];
      norm =  Dot[opk, opk];

      For[n = 1, n ≤ 4, n++,
       β[[4 * (j - 1) + k]][[4 * (m - 1) + n]] =
         Dot[opk, Flatten[opmstatej.nops[[n]]]] / norm;
      ]
     ]
    ]
   ];
   β
  ];
```

```
α = 1; -1;

opx = 1 * (σp + σm);
opy = (-ⅈ σp + ⅈ σm); (* -ⅈ* *)
opz = ( - σm.σp + σp.σm);
opi = ident[2];
opii = TensProd[opi, opi];
opxi = α * TensProd[opx, opi];
opyi = α * TensProd[opy, opi];
opzi = TensProd[opz, opi];

opix = α * TensProd[opi, opx];
opxx = α^2 * TensProd[opx, opx];
opyx = α * TensProd[opy, opx];
opzx = α * TensProd[opz, opx];

opiy = α * TensProd[opi, opy];
opxy = α^2 * TensProd[opx, opy];
opyy = α^2 * TensProd[opy, opy];
opzy = α * TensProd[opz, opy];

opiz = TensProd[opi, opz];
opxz = α * TensProd[opx, opz];
opyz = α * TensProd[opy, opz];
opzz = TensProd[opz, opz];
```

```
In[59]:= (* Make a two qubit density matrix with QId,
X90p, Y90p, or Xp rotations on both qubits *)
makeρ2[state_] := Module[{o1, o2},
   ρ = (σii + σiz + σzi + σzz) / 4; (* start from the ground state *)

   o1 = Switch[Characters[state][[1]],
     "I", U[0, σii],
     "X", U[π / 2, σxi],
     "Y", U[π / 2, σyi],
     "Z", U[π, σxi],
     _, U[0, σii]];
   o2 = Switch[Characters[state][[2]],
     "I", U[0, σii],
     "X", U[π / 2, σix],
     "Y", U[π / 2, σiy],
     "Z", U[π, σix],
     _, U[0, σii]];

   Return[dagger[o1].dagger[o2].ρ.o2.o1];
  ];

(* Programmatically create some order of states and operators *)
getorder2[] := Module[{basis, states, i, j, num},
   basis = {"I", "X", "Y", "Z"};
   states = Table[0, {16}];
```

```
   (* First programmatically create some order of states *)
   num = 1;
   For[i = 1, i ≤ Length[basis], i++,
    For[j = 1, j <= Length[basis], j++,
     states[[num]] = basis[[i]] <> basis[[j]];
     num++;
    ]
   ];
   states
  ];
states2 = getorder2[];
(* Give the density matrix of the kth state in our basis *)
state2[k_] := Module[{},
   (*states = getorder2[];*)
   makeρ2[states2[[k]]]
  ];
(* Give the jth operator in our basis *)
operator2[j_] := Module[{},
   (*states = getorder2[];
   ToExpression["σ"<>ToLowerCase[states2[[j]]]]*)
   ToExpression["op" <> ToLowerCase[states2[[j]]]]
  ];


(*ρ2[xi_,yi_,zi_,ix_,iy_,iz_,
   xy_,xz_,yx_,yz_,zx_,zy_,xx_,yy_,zz_] :=
  (σii+xi*σxi+yi*σyi+zi*σzi+ix*σix+xx*σxx+yx*σyz+zx*σzx+iy*σiy+
    xy*σxy+yy*σyy+zy*σzy+iz*σiz+xz*σxz+yz*σyz+zz*σzz);*)

paulitomo2[ρ_] := Table[Tr[ρ.operator2[ii]], {ii, 1, 16}] / 4;

get2Qλs[fullλ_] := Module[{α},
   λ = Table[0, {16}];

   α = -1;

   λ[[1]] = fullλ[[1]]; (* II *)
   λ[[2]] = α * fullλ[[5]]; (* IX *)
   λ[[3]] = α * fullλ[[6]]; (* IY *)
   λ[[4]] = fullλ[[7]]; (* IZ *)
   λ[[5]] = α * fullλ[[2]]; (* XI *)
   λ[[6]] = fullλ[[11]]; (* XX *)
   λ[[7]] = fullλ[[12]]; (* XY *)
   λ[[8]] = α * fullλ[[13]]; (* XZ *)
   λ[[9]] = α * fullλ[[3]]; (* YI *)
   λ[[10]] = fullλ[[14]]; (* YX *)
   λ[[11]] = fullλ[[15]]; (* YY *)
   λ[[12]] = α * fullλ[[16]]; (* YZ *)
   λ[[13]] = fullλ[[4]]; (* ZI *)
   λ[[14]] = α * fullλ[[17]]; (* ZX *)
```

```
  λ[[15]] = α * fullλ[[18]]; (* ZY *)
  λ[[16]] = fullλ[[19]]; (* ZZ *)

  λ
 ];

Calcβ2d[] := Module[
  {d, j, k, m, n, ii, β, opk, statej, opmstatej, norm, nops},
  d = 2 ^ 2;
  β = ConstantArray[0, {d ^ 4, d ^ 4}];

  nops = Table[0, {ii, 1, d ^ 2}];
  For[ii = 1, ii ≤ d ^ 2, ii ++,
   nops[[ii]] = operator2[ii];
  ];

  For[j = 1, j ≤ d ^ 2, j ++,
   statej = state2[j];
   (*Print[j];*)

   For[m = 1, m ≤ d ^ 2, m ++,
    opmstatej = operator2[m].statej;

    For[k = 1, k ≤ d ^ 2, k ++,
     opk = Flatten[operator2[k]];
     norm = Dot[opk, opk];

     For[n = 1, n ≤ d ^ 2, n ++,
      β[[d ^ 2 * (j - 1) + k]][[d ^ 2 * (m - 1) + n]] =
        Dot[opk, Flatten[opmstatej.dagger[nops[[n]]]]] / norm;
     ]
    ]
   ]
  ];
  β
 ];



Calcβ[j_, m_, k_, n_] := Module[{statej, opmstatej, opk, norm},

  statej = state2[j];
  opmstatej = operator2[m].statej;
  opk = Flatten[operator2[k]];
  norm = Dot[opk, opk];
  Print[norm];

  Dot[opk, Flatten[opmstatej.dagger[operator2[n]]]] / norm

 ];
```

# State Tomography

Here we show some examples of performing state tomography on states.

```
(* state tomography on the ground state |00> *)
paulibars = paulitomo2[state2[1]];
densitymatrix =
  Sum[paulibars[[ii]] * operator2[ii], {ii, 1, 16}];

BarChart[4 * paulibars, PlotRange → {-1, 1}]

GraphicsRow[{
  BarChart3D[Re[Normal[densitymatrix]],
   PlotRange -> {All, All, {-1.01, 1.01}}] ,
  BarChart3D[Im[Normal[densitymatrix]],
   PlotRange -> {All, All, {-1.01, 1.01}}]
 }]
```

Out[92]=

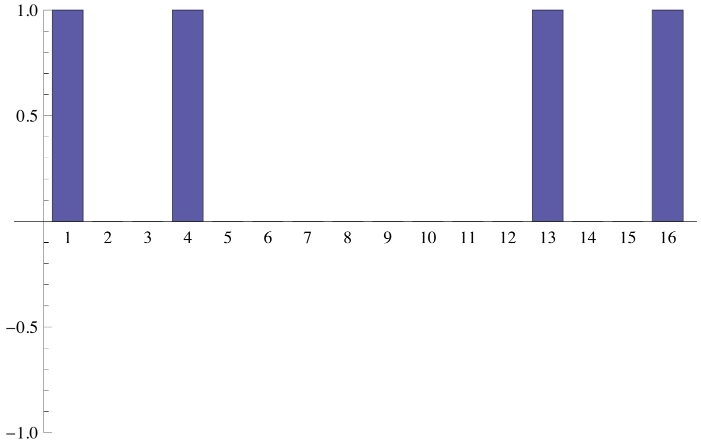


Out[93]=

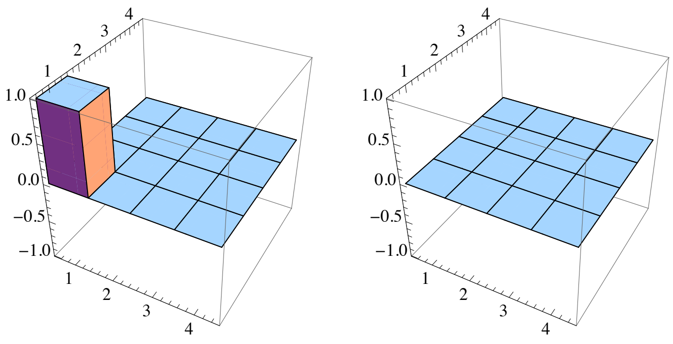

```
 (* state 16 is both qubits excited |11> *)
paulibars = paulitomo2[state2[16]];

BarChart[4 * paulibars, PlotRange → {-1, 1}]

GraphicsRow[{
  BarChart3D[Re[Normal[densitymatrix]],
   PlotRange -> {All, All, {-1.01, 1.01}}] ,
  BarChart3D[Im[Normal[densitymatrix]],
   PlotRange -> {All, All, {-1.01, 1.01}}]
 }]
```

Out[95]=

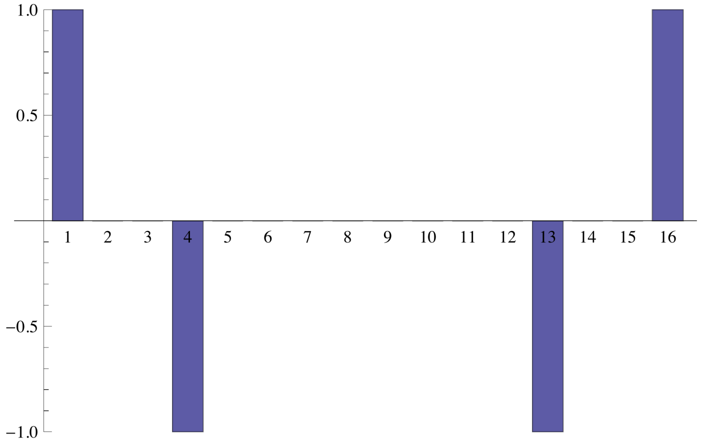


Out[96]=

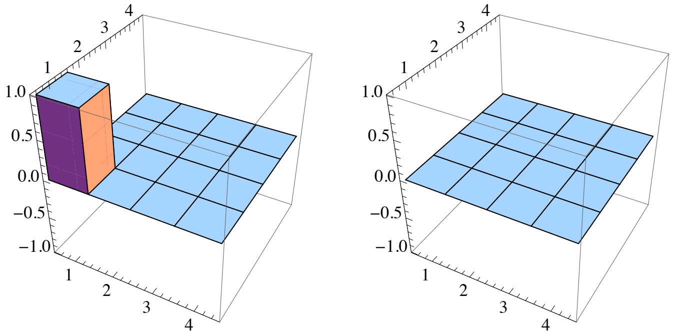

```
(* State tomography on a Bell state *)
phasegate = DiagonalMatrix[
   {1, Exp[I * (ϕ01)], Exp[I * (ϕ10)], Exp[I * (ϕ01 + ϕ10 + ϕ11)]}];
cphase = phasegate /. {ϕ01 → 0, ϕ10 → 0, ϕ11 → π};

(* Circuit to create a Bell state from the ground state *)
bellproc = U[-π / 2, σyi].U[-π / 2, σiy].cphase.U[π / 2, σyi];

states2 = {"II", "XI", "YI", "ZI", "IX", "IY", "IZ", "XX", "XY",
  "XZ", "YX", "YY", "YZ", "ZX", "ZY", "ZZ"}; getorder2[];

paulibars = paulitomo2[dagger[bellproc].makeρ2["II"].bellproc];
BarChart[4 * paulibars, PlotRange → {-1, 1}]
```

Out[102]=

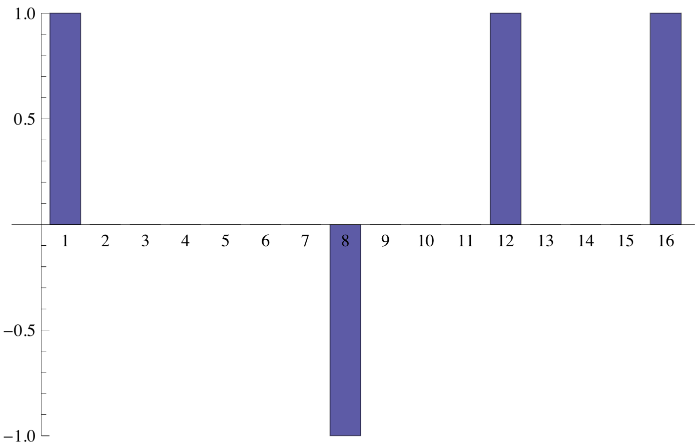


```
(* Compare this to some random experimentally-
 measured Bell state and calculate the fidelity *)
exptData = {1, 0.082, -0.053, 0.037, 0.036, 0.009, 0.021,
   -0.804, .152, -.079, .197, .793, .047, -.007, .079, .959};
BarChart[exptData, PlotRange → {-1, 1}]
Sum[paulibars[[ii]] * exptData[[ii]], {ii, 1, 16}]
```

Out[106]=

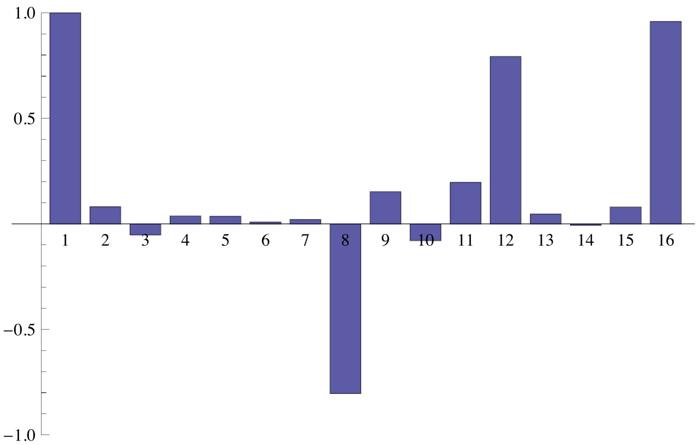


Out[107]= 0.889

```
(* Try to match up the data with a process with different single-
 qubit phases to optimize the fidelity. *)
testSQAngles[ϕ01angle_, ϕ10angle_, ϕ11angle_, exptData_] :=
  Module[{phasegate, cphase, bellproc, states2, paulibars},
   phasegate = DiagonalMatrix[
     {1, Exp[I * (ϕ01)], Exp[I * (ϕ10)], Exp[I * (ϕ01 + ϕ10 + ϕ11)]}];
   cphase = phasegate /. {ϕ01 → ϕ01angle * π / 180,
      ϕ10 → ϕ10angle * π / 180 , ϕ11 → π + ϕ11angle * π / 180};

   bellproc = U[-π / 2, σyi].U[-π / 2, σiy].cphase.U[π / 2, σyi];

   states2 =
    {"II", "XI", "YI", "ZI", "IX", "IY", "IZ", "XX", "XY",
     "XZ", "YX", "YY", "YZ", "ZX", "ZY", "ZZ"}; getorder2[];

   paulibars =
    paulitomo2[dagger[bellproc].makeρ2["II"].bellproc];

   Re[Sum[paulibars[[ii]] * exptData[[ii]], {ii, 1, 16}]]

  ];
```

```
In[108]:= testSQAngles[20, 0, 0, exptData]

Out[108]= 0.894764
```

```
In[109]:= FindMaximum[testSQAngles[x, y, z, exptData],
  {{x, 0}, {y, 0}, {z, 0}}]
```

FindMaximum::lstol :
The line search decreased the step size to within the tolerance specified by AccuracyGoal and PrecisionGoal but was unable to find a sufficient increase in the function. You may need more than MachinePrecision digits of working precision to meet these tolerances. ≫

```
Out[109]= {0.898571, {x → 11.1311, y → -2.06128, z → 2.31932}}
```

# Two-qubit Process Tomography

Code to create the $\beta$ matrix for converting state tomography data into a $\chi$ matrix.

```
AbsoluteTiming[β2 = Calcβ2d[];]
AbsoluteTiming[κ2 = Inverse[N[β2]];]

CNot = {{1, 0, 0, 0}, {0, 1, 0, 0}, {0, 0, 0, 1}, {0, 0, 1, 0}};

CPhase = {{1, 0, 0, 0}, {0, 1, 0, 0}, {0, 0, 1, 0}, {0, 0, 0, -1}};

Out[68]= {2.753845, Null}

Out[69]= {0.063325, Null}
```

```
(* Process tomography on the identity
 just to verify that everything isn't crazy *)
Proc = U[0, σii];
λ2 =
  Table[paulitomo2[Proc.state2[ii].dagger[Proc]], {ii, 1, 16}];
χ2 = Partition[κ2.Flatten[λ2], 16];

GraphicsRow[{
  BarChart3D[Re[χ2], PlotRange -> {All, All, {-1.01, 1.01}}] ,
  BarChart3D[Im[χ2], PlotRange -> {All, All, {-1.01, 1.01}}]
 }]
```

Out[81]=

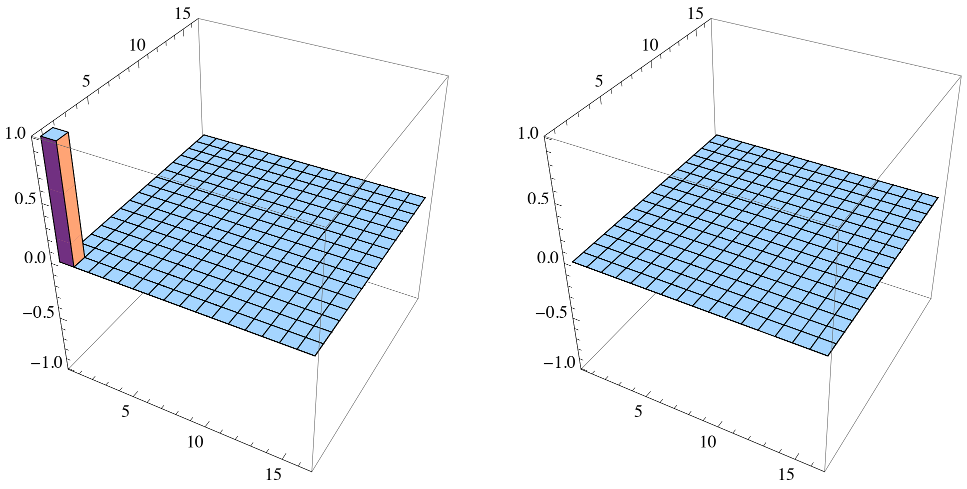

```
(* Proc tomo on the cNOT gate *)
Proc = CNot;
λ2 =
  Table[paulitomo2[Proc.state2[ii].dagger[Proc]], {ii, 1, 16}];
χ2 = Partition[κ2.Flatten[λ2], 16];
(*χ2 //MatrixForm*)

GraphicsRow[{
  BarChart3D[Re[χ2], PlotRange -> {All, All, {-0.251, 0.251}}] ,
  BarChart3D[Im[χ2], PlotRange -> {All, All, {-0.251, 0.251}}]
 }]
```

Out[77]=

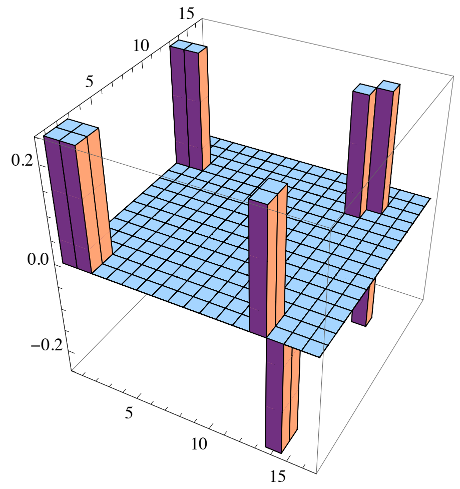


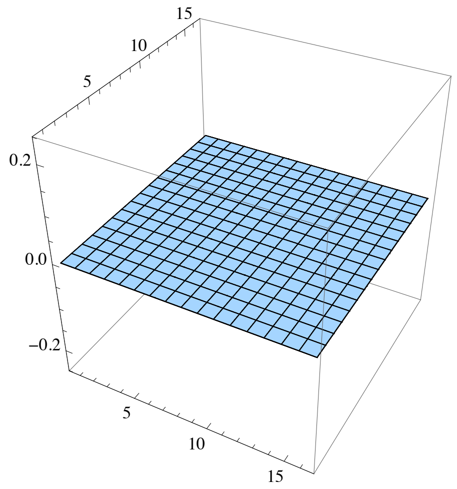

```
(* cPhase gate tomo *)
Proc = CPhase;
λ2 =
  Table[paulitomo2[Proc.state2[ii].dagger[Proc]], {ii, 1, 16}];
χ2 = Partition[κ2.Flatten[λ2], 16];
(*χ2 //MatrixForm*)

GraphicsRow[{
  BarChart3D[Re[χ2], PlotRange -> {All, All, {-0.26, 0.26}}] ,
  BarChart3D[Im[χ2], PlotRange -> {All, All, {-1, 1}}]
 }]
```

Out[85]=

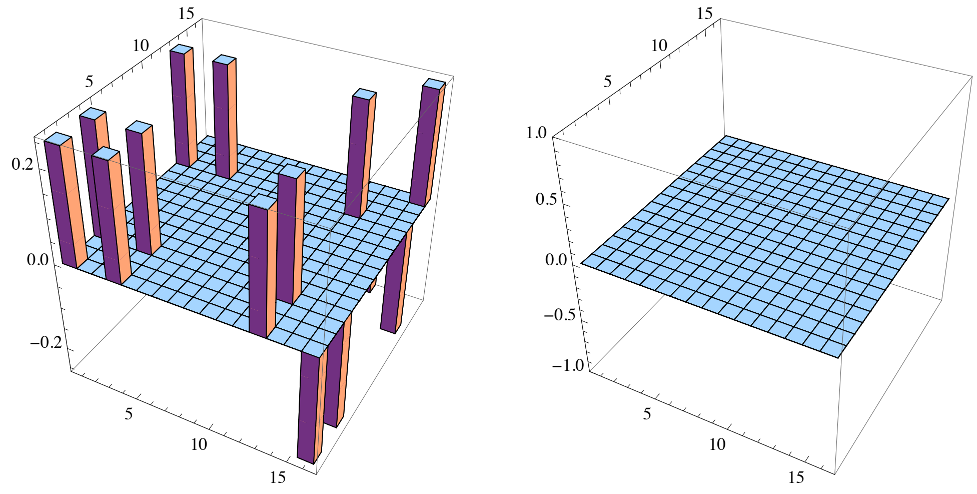

```
(* ZZ gate *)
Proc = U[π / 2, σzz];
λ2 =
  Table[paulitomo2[Proc.state2[ii].dagger[Proc]], {ii, 1, 16}];
χ2 = Partition[ϰ2.Flatten[λ2], 16];
(*χ2 //MatrixForm*)

GraphicsRow[{
  BarChart3D[Re[χ2], PlotRange -> {All, All, {-0.51, 0.51}}] ,
  BarChart3D[Im[χ2], PlotRange -> {All, All, {-0.51, 0.51}}]
 }]
```

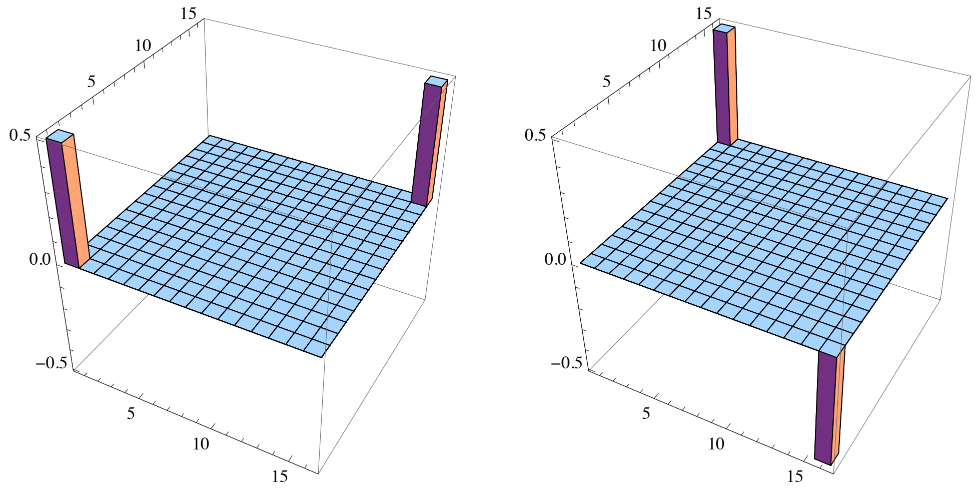


# AllXY Syndromes

Define the AllXY sequence with parameters of certain error syndromes. Import data and calculate the syndromes, and see that they're the same! In the mean time, we will also analytically calculate the leading-order dependence of each sequence to whichever error.

In[119]:=
```
Δ = (-11 + jj) * 10^6;
δt  =  9 * 10^-9;
xscale = 1;
```

```
In[117]:= zProj[operator_] := Tr[operator.state1[1].dagger[operator].σz];

GetAllXY[rs_, Δ_, δt_, xscale_] := Module[{},

    Δop = -2 π * Δ * δt * σz;

    {
     {U[π, σi + Δop / π], U[π, σi + Δop / π]},
     {U[π, rs * xscale * σx + Δop / π], U[π, rs * xscale * σx + Δop / π]},
     {U[π, rs * σy + Δop / π], U[π, rs * σy + Δop / π]},
     {U[π, rs * xscale * σx + Δop / π], U[π, rs * σy + Δop / π]},
     {U[π, rs * σy + Δop / π], U[π, rs * xscale * σx + Δop / π]},

     {U[π / 2, rs * xscale * σx + Δop / (π / 2)], U[π, σi + Δop / π]},
     {U[π / 2, rs * σy + Δop / (π / 2)], U[π, σi + Δop / π]},
     {U[π / 2, rs * xscale * σx + Δop / (π / 2)],
      U[π / 2, rs * σy + Δop / (π / 2)]}, {U[π / 2, rs * σy + Δop / (π / 2)],
      U[π / 2, rs * xscale * σx + Δop / (π / 2)]},
     {U[π / 2, rs * xscale * σx + Δop / (π / 2)], U[π, rs * σy + Δop / π]},
     {U[π / 2, rs * σy + Δop / (π / 2)], U[π, rs * xscale * σx + Δop / π]},

     {U[π, rs * xscale * σx + Δop / π], U[π / 2, rs * σy + Δop / (π / 2)]},
     {U[π, rs * σy + Δop / π], U[π / 2, rs * xscale * σx + Δop / (π / 2)]},

     {U[π / 2, rs * xscale * σx + Δop / (π / 2)],
      U[π, rs * xscale * σx + Δop / π]}, {U[π, rs * xscale * σx + Δop / π],
      U[π / 2, rs * xscale * σx + Δop / (π / 2)]},
     {U[π / 2, rs * σy + Δop / (π / 2)], U[π, rs * σy + Δop / π]},
     {U[π, rs * σy + Δop / π], U[π / 2, rs * σy + Δop / (π / 2)]},

     {U[π, rs * σy + Δop / π], U[π, σi + Δop / π]},
     {U[π, rs * σy + Δop / π], U[π, σi + Δop / π]},
     {U[π / 2, rs * xscale * σx + Δop / (π / 2)],
      U[π / 2, rs * xscale * σx + Δop / (π / 2)]},
     {U[π / 2, rs * σy + Δop / (π / 2)], U[π / 2, rs * σy + Δop / (π / 2)]}
    }];
```

In[122]:=
```
rs = (1.1); (* rotation angle scaling *)
Δ = 0 * 11 * 10^6;
δt = 8 * 10^-9;
xscale = 1;
AllXY = GetAllXY[rs, Δ, δt, xscale];

ListLinePlot[Chop[Table[zProj[AllXY[[Ceiling[ii / 2]]][[1]].
      AllXY[[Ceiling[ii / 2]]][[2]]], {ii, 1, 2 * 21}]]]
```

Out[127]=

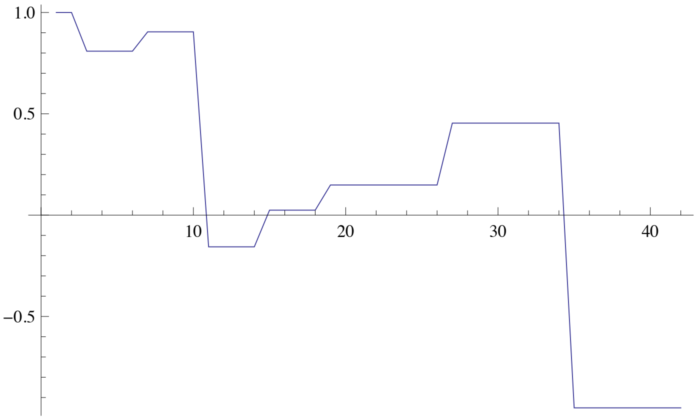


## Calculate leading – order power dependence

In[128]:=
```
rs = (1 + ϵ);
Δ = 0 * 10^6;
δt = 8 * 10^-9;
xscale = 1;
AllXYPowerEps = GetAllXY[rs, Δ, δt, xscale];
Chop[
  Series[
   FullSimplify[
     Table[zProj[AllXYPowerEps[[ii]][[1]].
        AllXYPowerEps[[ii]][[2]]], {ii, 1, 21}]
     , {Element[ϵ, Reals]}] /. {ϵ → ϵ / π * 2}, {ϵ, 0, 4}]] //
 MatrixForm
```

Out[133]//MatrixForm=

$$\begin{pmatrix} 1 \\ 1 - 8\epsilon^2 + \frac{32\epsilon^4}{3} + O[\epsilon]^5 \\ 1 - 8\epsilon^2 + \frac{32\epsilon^4}{3} + O[\epsilon]^5 \\ 1 - 4\epsilon^2 + \frac{16\epsilon^4}{3} + O[\epsilon]^5 \\ 1 - 4\epsilon^2 + \frac{16\epsilon^4}{3} + O[\epsilon]^5 \\ -\epsilon + \frac{\epsilon^3}{6} + O[\epsilon]^5 \\ -\epsilon + \frac{\epsilon^3}{6} + O[\epsilon]^5 \\ \epsilon^2 - \frac{\epsilon^4}{3} + O[\epsilon]^5 \\ \epsilon^2 - \frac{\epsilon^4}{3} + O[\epsilon]^5 \\ \epsilon - \frac{13\epsilon^3}{6} + O[\epsilon]^5 \\ \epsilon - \frac{13\epsilon^3}{6} + O[\epsilon]^5 \\ \epsilon - \frac{13\epsilon^3}{6} + O[\epsilon]^5 \\ \epsilon - \frac{13\epsilon^3}{6} + O[\epsilon]^5 \\ 3\epsilon - \frac{9\epsilon^3}{2} + O[\epsilon]^5 \\ 3\epsilon - \frac{9\epsilon^3}{2} + O[\epsilon]^5 \\ 3\epsilon - \frac{9\epsilon^3}{2} + O[\epsilon]^5 \\ 3\epsilon - \frac{9\epsilon^3}{2} + O[\epsilon]^5 \\ -1 + 2\epsilon^2 - \frac{2\epsilon^4}{3} + O[\epsilon]^5 \\ -1 + 2\epsilon^2 - \frac{2\epsilon^4}{3} + O[\epsilon]^5 \\ -1 + 2\epsilon^2 - \frac{2\epsilon^4}{3} + O[\epsilon]^5 \\ -1 + 2\epsilon^2 - \frac{2\epsilon^4}{3} + O[\epsilon]^5 \end{pmatrix}$$

## Calculate leading – order detuning dependence

In[134]:=
```
rs = (1);
Δ = ϵ;
δt = 1;
xscale = 1;
AllXYDeltaEps = GetAllXY[rs, Δ, δt, xscale];

Collect[Simplify[Normal[Series[Simplify[ComplexExpand[Table[
        zProj[
         AllXYDeltaEps[[ii]][[1]].AllXYDeltaEps[[ii]][[2]]]
        , {ii, 1, 21}]], {ϵ > 0}], {ϵ, 0, 4}]]], ϵ] /. {ϵ → ϵ / 4} //
  MatrixForm
```

Out[139]//MatrixForm=

$$\begin{pmatrix}
1 \\
1-\frac{\pi^2 \epsilon^4}{32} \\
1-\frac{\pi^2 \epsilon^4}{32} \\
1-\epsilon^2-\frac{\pi \epsilon^3}{4}-\frac{1}{64}\left(-32+\pi^2\right)\epsilon^4 \\
1-\epsilon^2+\frac{\pi \epsilon^3}{4}-\frac{1}{64}\left(-32+\pi^2\right)\epsilon^4 \\
\frac{1}{16}(16-4\pi)\epsilon^2+\frac{1}{16}(-16+5\pi)\epsilon^4 \\
\frac{1}{16}(16-4\pi)\epsilon^2+\frac{1}{16}(-16+5\pi)\epsilon^4 \\
2\epsilon+\frac{1}{2}(-6+\pi)\epsilon^3+\frac{1}{16}(-4+\pi)^2\epsilon^4 \\
-2\epsilon-\frac{1}{2}(-6+\pi)\epsilon^3+\frac{1}{16}(-4+\pi)^2\epsilon^4 \\
\epsilon+\frac{1}{4}(-4+\pi)\epsilon^2-\frac{1}{8}(6+\pi)\epsilon^3-\frac{1}{16}(-24+7\pi)\epsilon^4 \\
-\epsilon+\frac{1}{4}(-4+\pi)\epsilon^2+\frac{1}{8}(6+\pi)\epsilon^3-\frac{1}{16}(-24+7\pi)\epsilon^4 \\
\epsilon+\frac{1}{4}(-4+\pi)\epsilon^2-\frac{1}{8}(6+\pi)\epsilon^3-\frac{1}{16}(-24+7\pi)\epsilon^4 \\
-\epsilon+\frac{1}{4}(-4+\pi)\epsilon^2+\frac{1}{8}(6+\pi)\epsilon^3-\frac{1}{16}(-24+7\pi)\epsilon^4 \\
\frac{3\pi\epsilon^2}{8}+\frac{1}{256}(64-70\pi)\epsilon^4 \\
\frac{3\pi\epsilon^2}{8}+\frac{1}{256}(64-70\pi)\epsilon^4 \\
\frac{3\pi\epsilon^2}{8}+\frac{1}{256}(64-70\pi)\epsilon^4 \\
\frac{3\pi\epsilon^2}{8}+\frac{1}{256}(64-70\pi)\epsilon^4 \\
-1+\frac{\epsilon^2}{2}+\frac{1}{128}\left(-16+\pi^2\right)\epsilon^4 \\
-1+\frac{\epsilon^2}{2}+\frac{1}{128}\left(-16+\pi^2\right)\epsilon^4 \\
-1+2\epsilon^2+\frac{1}{8}\left(-16+\pi^2\right)\epsilon^4 \\
-1+2\epsilon^2+\frac{1}{8}\left(-16+\pi^2\right)\epsilon^4
\end{pmatrix}$$

```
(* Import actual data and find that
 they're the same to our expectations *)
allxypow = Transpose[
   Drop[Import["~/Desktop/Thesis/SingleQubitGates/allxy
        syndromes/allxy_pow_table.txt", {"Table"}], 2]];

allxypownorm = -2 *
     (allxypow - Min[allxypow]) / (Max[allxypow] - Min[allxypow]) + 1;
allxypownorm = 2 * (allxypow - allxypow[[11]][[37]]) /
      (allxypow[[11]][[1]] - allxypow[[11]][[37]]) - 1;

ListLinePlot[allxypownorm]
```

Out[143]=

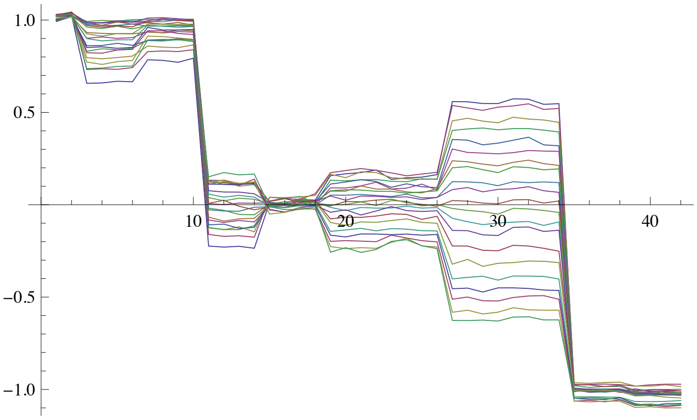

In[144]:=
```
allxydelta =
  Transpose[Drop[Import["~/Desktop/Thesis/SingleQubitGates/allxy
      syndromes/allxy_delta_table.txt", {"Table"}], 2]];

allxydeltanorm = -2 * (allxydelta - Min[allxydelta]) /
    (Max[allxydelta] - Min[allxydelta]) + 1;
allxydeltanorm = 2 * (allxydelta - allxydelta[[11]][[37]]) /
    (allxydelta[[11]][[1]] - allxydelta[[11]][[37]]) - 1;



ListLinePlot[allxydeltanorm]
```

Out[147]=

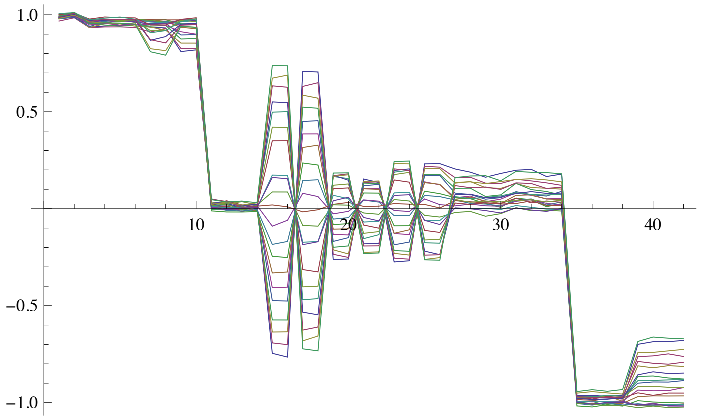


```
rs = 10^(0.9 / 20.); (1.14); (* rotation angle scaling *)
Δ = 0 * 11 * 10^6;
δt = 8 * 10^-9;
xscale = 1;
AllXY = GetAllXY[rs, Δ, δt, xscale];

ListLinePlot[{Table[zProj[
    AllXY[[Ceiling[ii / 2]]][[1]].AllXY[[Ceiling[ii / 2]]][[2]]],
   {ii, 1, 2 * 21}], allxypownorm[[2]]}]
```

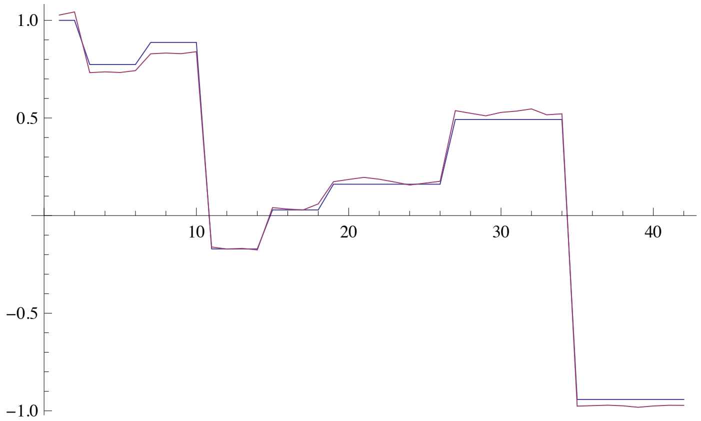

In[148]:=
```
Table[

 rs = 10^((1.1 - jj / 10) / 20.);
 (1.14); (* rotation angle scaling *)
 Δ = 0 * 11 * 10^6;
 δt  = 8 * 10^-9;
 xscale = 1;
 AllXY = GetAllXY[rs, Δ, δt, xscale];

 ListLinePlot[{Table[zProj[
      AllXY[[Ceiling[ii / 2]]][[1]].AllXY[[Ceiling[ii / 2]]][[2]]],
    {ii, 1, 2 * 21}], allxypownorm[[jj]]}],

 {jj, 1, 21}]
```

Out[148]= {

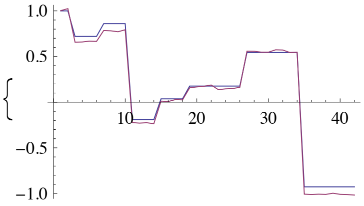

,

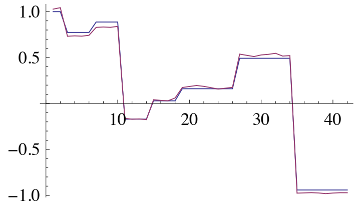

,

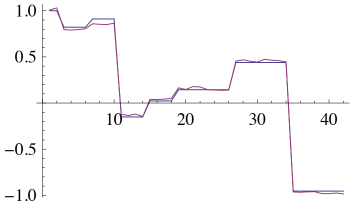

,

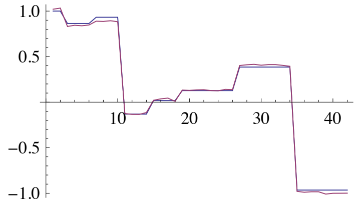

,

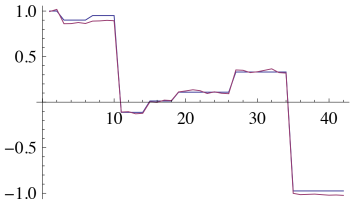

,

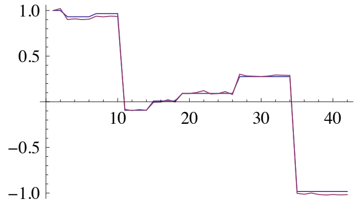

,

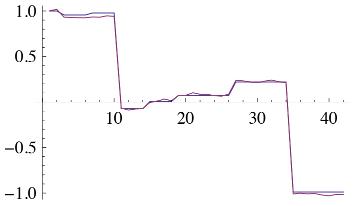

,

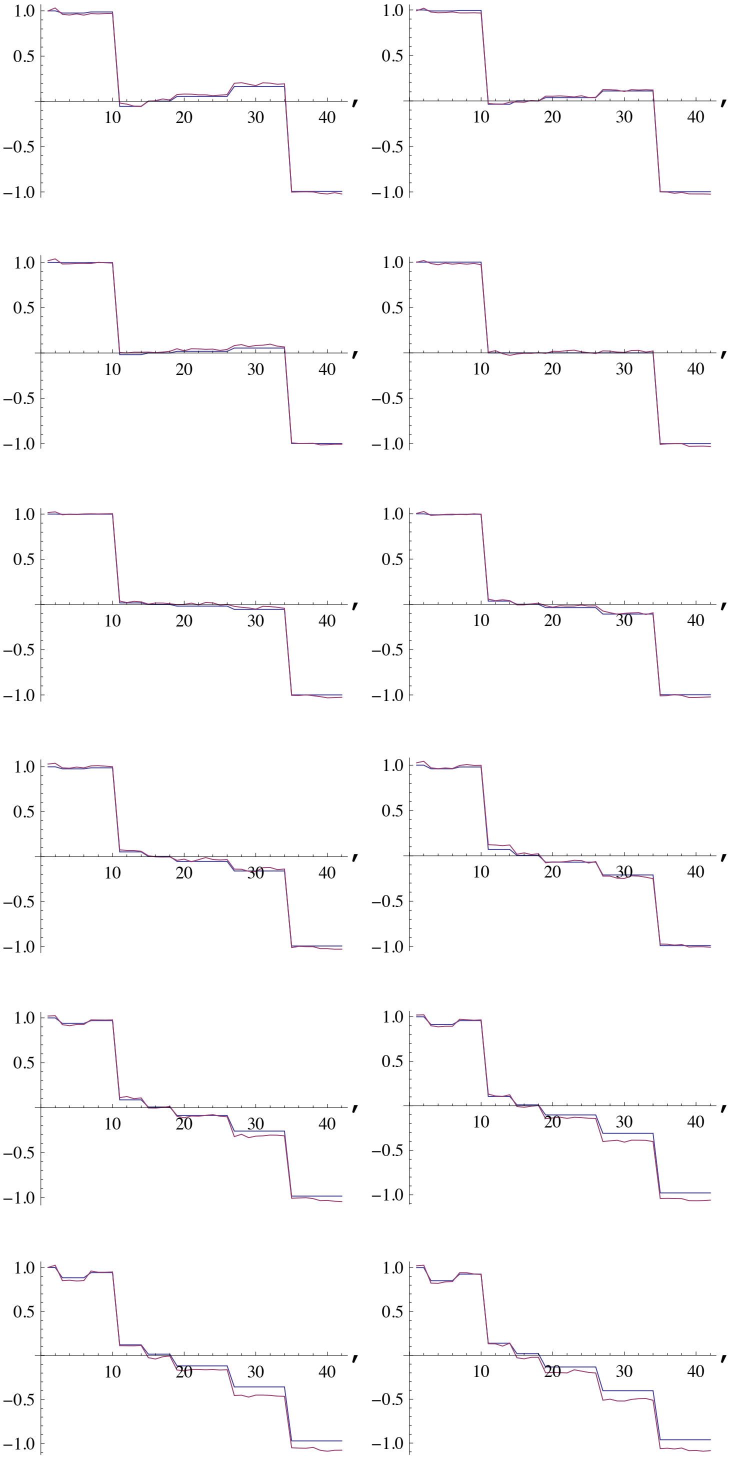
1.0
0.5
−0.5
−1.0
10
20
30
40

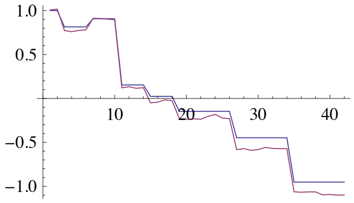


,

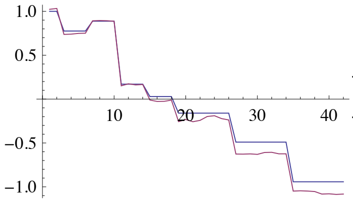


}

In[149]:=
```
Export["amplitude.txt", Chop[N[Table[
    rs = 10^((1.1 - jj / 10) / 20.);
    (1.14); (* rotation angle scaling *)
    Δ = 0 * 11 * 10^6;
    δt = 8 * 10^-9;
    xscale = 1;
    AllXY = GetAllXY[rs, Δ, δt, xscale];

    Table[zProj[AllXY[[Ceiling[ii / 2]]][[1]].
       AllXY[[Ceiling[ii / 2]]][[2]]], {ii, 1, 2 * 21}],

    {jj, 1, 21}]]]]
```

Out[149]= amplitude.txt

In[150]:=
```
Table[
 rs = 1; (* rotation angle scaling *)
 Δ = (-11 + jj) * 10^6;
 δt = 9 * 10^-9;
 xscale = 1;
 AllXY = GetAllXY[rs, Δ, δt, xscale];

 ListLinePlot[{Table[zProj[
     AllXY[[Ceiling[ii / 2]]][[1]].AllXY[[Ceiling[ii / 2]]][[2]]],
    {ii, 1, 2 * 21}], allxydeltanorm[[jj]]}],

 {jj, 1, 21}]
```

Out[150]= {

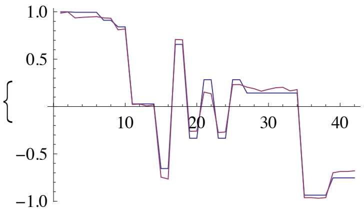


,

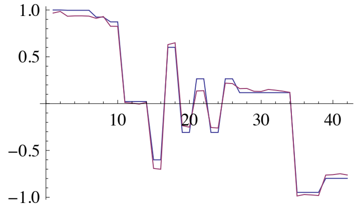


,

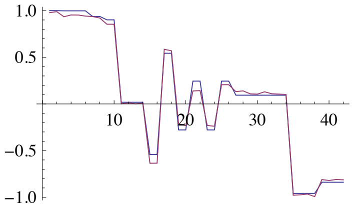


,

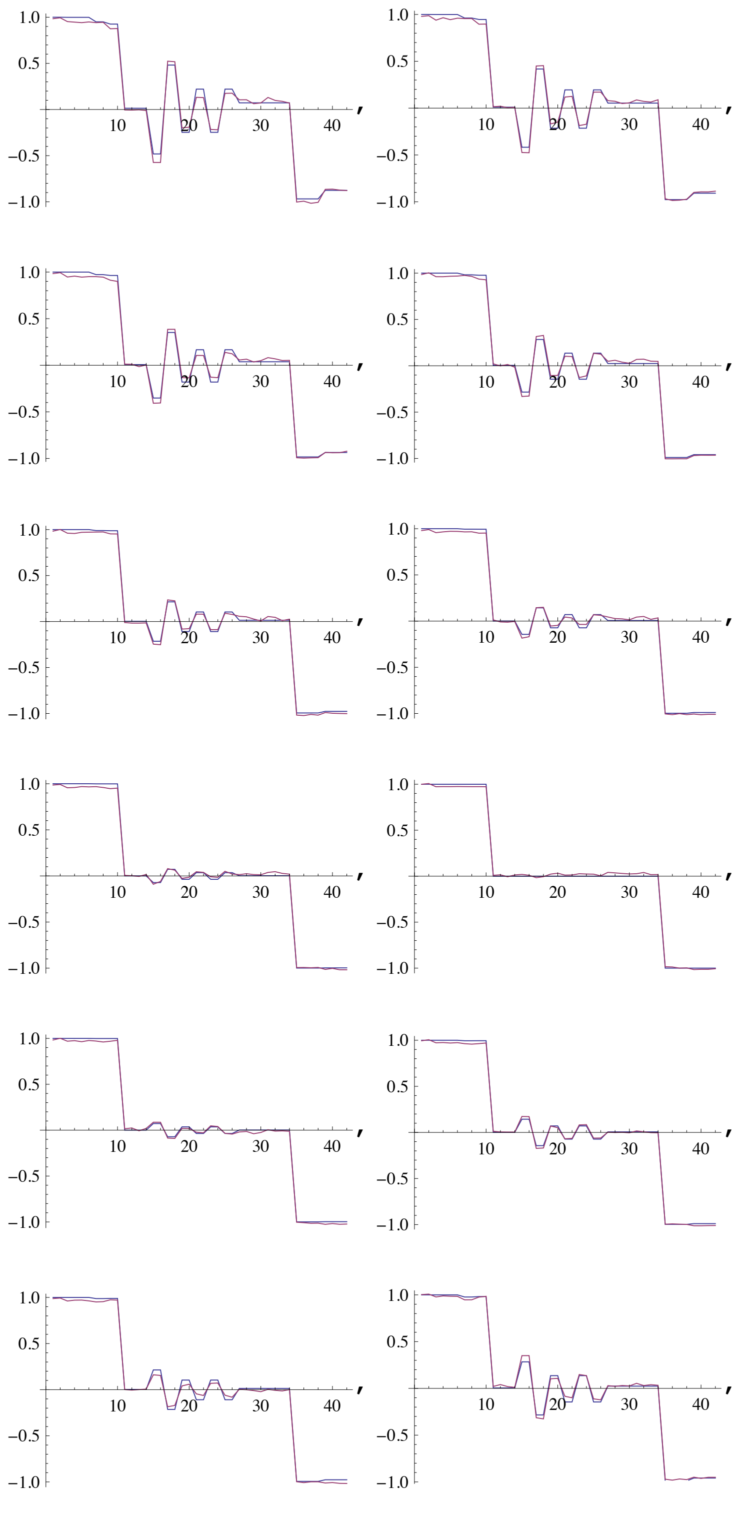
1.0
0.5
10
20
30
40
−0.5
−1.0

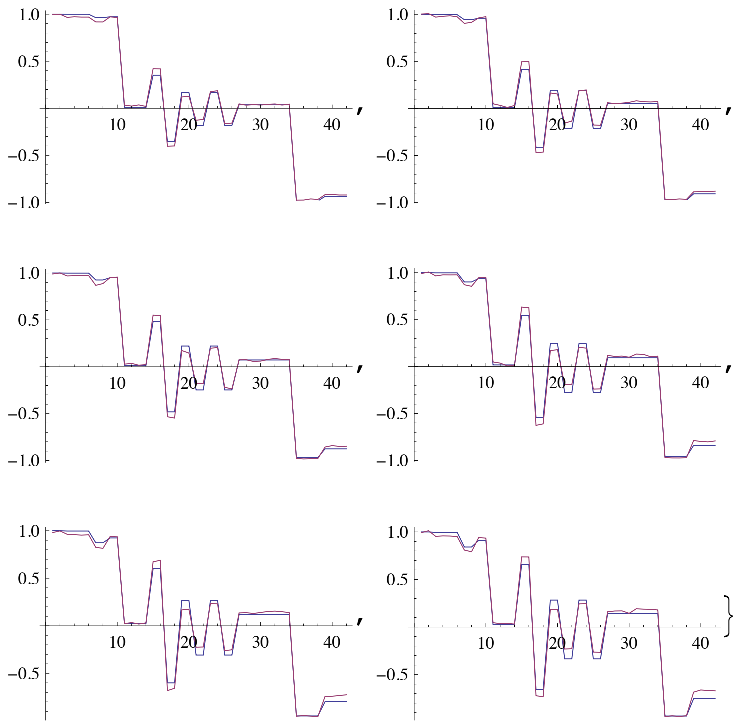


In[151]:=
```
Export["detuning.txt", Chop[N[Table[
    rs = 1; (* rotation angle scaling *)
    Δ = (-11 + jj) * 10^6;
    δt = 9 * 10^-9;
    xscale = 1;
    AllXY = GetAllXY[rs, Δ, δt, xscale];

    Table[zProj[AllXY[[Ceiling[ii / 2]]][[1]].
       AllXY[[Ceiling[ii / 2]]][[2]]], {ii, 1, 2 * 21}],

    {jj, 1, 21}]]]]
```
Out[151]= detuning.txt

In[153]:=
```
Export["xscale.txt",
 Chop[N[Table[rs = 1; (* rotation angle scaling *)
    Δ = 0 * 11 * 10^6;
    δt = 8 * 10^-9;
    xscale = (0.96 + jj / 100) / 1.02 ;
    AllXY = GetAllXY[rs, Δ, δt, xscale];

    Table[zProj[AllXY[[Ceiling[ii / 2]]][[1]].
       AllXY[[Ceiling[ii / 2]]][[2]]], {ii, 1, 2 * 21}],

    {jj, 0, 11}]]]]
```
Out[153]= xscale.txt
