# Supplementary material for: Entanglement and Quantum Error Correction with Superconducting Qubits
Source: arXiv:1311.6759 source file (2013-11-26)
Supplement: Supplementary file 2 [file startappendices.tex]

\appendix
\cleardoublepage
\oldphantomsection
\addcontentsline{toc}{part}{Appendices}
%..."part" means Appendices are child of this in outline (good) but also means backmatter is children of this (maybe not good)
%This file exists as its own include file to force it to come ahead of the actual appendices in the ToC! (Due to \immediate vs non-\immediate write-related crap)
% \usepackage{appendix}, maybe useful? (But it seems to have same problem...)
